# Supplementary material for: Electron pumping in graphene mechanical resonators
Source: arXiv:1203.0348 source file (2012-03-02)
Supplement: Supplementary file 1 [file supplinfo.pdf]

## Supplementary Information: Electron pumping in graphene mechanical resonators

T. Low<sup>1</sup>, Y. J. Jiang<sup>2,3</sup>, M. I. Katsnelson<sup>4</sup>, and F. Guinea<sup>5</sup>

<sup>1</sup> *IBM T.J. Watson Research Center, Yorktown Heights, NY 10598, USA*

<sup>2</sup> *Department of Physics, ZheJiang Normal University, Zhejiang 321004, People's Republic of China*

<sup>3</sup> *Department of Physics, Purdue University, West Lafayette, Indiana 47909, USA*

<sup>4</sup> *Radboud University Nijmegen, Institute for Molecules and Materials,  
Heyendaalseweg 135, 6525AJ Nijmegen, The Netherlands*

<sup>5</sup> *Instituto de Ciencia de Materiales de Madrid. CSIC. Sor Juana Inés de la Cruz 3. 28049 Madrid, Spain*

We consider a suspended graphene resonator as described in [1, 2]. The dynamical equation for the out-of-plane deformation from equilibrium  $a(t)$  is given by (see the respective Appendixes on the form of the forces),

$$\rho \frac{\partial^2 a}{\partial t^2} = \mathcal{F}_S + \mathcal{F}_D + \mathcal{F}_E \quad (1)$$

where  $\mathcal{F}_S$ ,  $\mathcal{F}_D$ ,  $\mathcal{F}_E$  are the time dependent restoring elastic, damping and electrostatic forces (or pressures) respectively, in units of  $m^{-2}$ .  $\rho$  is the mass density. The total restoring elastic force, ignoring second order terms due to bending forces  $\kappa$  and  $O(h^2)$ , reduces to,

$$\mathcal{F}_S = -\frac{64}{3} \frac{\lambda + 2\mu}{L^4} (a^3 + 3a^2 h_0 + 3a h_0^2) + \frac{8\Delta L}{L^3} (\lambda + 2\mu) a \quad (2)$$

obtained by minimizing elastic energy. Damping is treated phenomenologically via,

$$\mathcal{F}_D = -\frac{\rho}{\tau_d} \frac{\partial a}{\partial t} \quad (3)$$

$\tau_d$  can be easily obtained from quality factor  $Q$  measured in experiments.  $Q$  is defined to be  $Q = \omega_0 / \Delta\omega = \omega_0 \tau_d / 2$ , where  $\Delta\omega$  is the so called bandwidth of the resonance peak. Reported  $Q$  is around 100 [1, 2] at room temperature, depending on many factors. For example, temperature dependence of  $Q \propto T^{-0.36}$  was found, for  $T < 100K$  [2]. And a record  $Q \approx 100,000$  at  $90mK$  was reported [3]. Mass density of graphene assumed to be  $\rho \approx 7.4 \times 10^{-6} kgm^{-2}$ . Lastly, the electrostatic force is modelled as,

$$\mathcal{F}_E = \frac{C_T^2 V_{dc} V_{ac}}{\epsilon_0} \cos(\omega t) \quad (4)$$

neglecting  $O(V_{ac}^2)$  and other non-linear terms.  $C_T = [\epsilon_0^{-1}(d + h_0) + \epsilon_{SiO_2}^{-1} t_{SiO_2}]^{-1}$  is the total effective capacitance due to the back-gate oxide and air dielectric,  $d$  being the perpendicular distance of the unstrained graphene from the substrate.

We are interested in the steady state solution to the dynamical equation i.e.  $a(\omega) = |a| \exp(i\phi)$ . We seek an approximate solution through an iterative technique used in the Duffing model [4, 5]. For convenience, we rewrite the dynamical equation as,

$$\rho \ddot{a} = -k_0 a - k_1 a^2 - k_2 a^3 - \frac{\rho}{\tau_d} \dot{a} + f \cos(\omega t) \quad (5)$$

where

$$k_0 = \frac{64(\lambda + 2\mu)h_0^2}{L^4} - \frac{8\Delta L}{L^3}(\lambda + 2\mu), \quad k_1 = \frac{64(\lambda + 2\mu)h_0}{L^4}, \quad k_2 = \frac{64(\lambda + 2\mu)}{3L^4}, \quad f = \frac{C_T^2 V_{dc} V_{ac}}{\epsilon_0} \quad (6)$$

In the spring constant term  $k_0$ , we consider only the case for  $\Delta L \leq 0$ .  $k_2$  contributes to the Duffing force, and renders the spring more stiff (soft) if positive (negative). In the former, the effect will be a shift of resonance with increasing driving force. And at larger driving force would lead to bistability and hysteresis [2].

The frequency response  $a(\omega)$  around the resonant frequency  $\omega_0 \equiv \sqrt{k_0/\rho}$  has the following approximate solution,

$$\left[ (\omega_0^2 - \omega^2)|a| + \frac{3k_2}{4\rho}|a|^3 \right]^2 + \left( \frac{\omega|a|}{\tau_d} \right)^2 = \left( \frac{f}{\rho} \right)^2 \quad (7)$$

$$\tan\phi = \frac{\omega|a|}{\tau_d \left[ (\omega_0^2 - \omega^2)|a| + \frac{3k_2}{4\rho}|a|^3 \right]} \quad (8)$$

Note that  $a^2$  terms affects the higher harmonics  $2\omega_0$ . These converge to the Lorentz model solutions if we set  $k_2 = 0$ . In the linear regime, i.e.  $k_2 = 0$ , the response at  $\omega = \omega_0$  goes as  $|a| = 2Qf/\rho\omega_0^2$ . When  $k_2 \neq 0$ ,  $|a|$  follows,

$$\frac{9k_2^2}{16}|a|^6 + \frac{k_0^2}{4Q^2}|a|^2 = f^2 \quad (9)$$

From this, we can define a threshold driving force  $f_{th}$  where  $|a(\omega = \omega_0)|$  starts to deviate from linearity i.e.  $|a| \propto f$ ,

$$f_{th} \approx \sqrt{\frac{k_0^3}{36Q^3k_2}} \quad (10)$$

As evident,  $\rho$  has no effect on  $f_{th}$ , and a larger  $Q$  yields a smaller  $f_{th}$  i.e. increased sensitivity to non-linearity. However, a larger  $Q$  is desirable to achieve a larger resonance  $|a(\omega = \omega_0)|$ .

## APPENDIX A: ELECTROSTATIC FORCES

The electrostatic force is modelled as,

$$\mathcal{F}_E^{tot} = \frac{1}{2} \frac{C_T^2}{\epsilon_0} V_{bg}^2 \approx \frac{1}{2} \frac{C_T^2}{\epsilon_0} (V_{dc}^2 + 2V_{dc}V_{ac}\cos(\omega t)) \equiv \mathcal{F}_E^{eq} + \mathcal{F}_E \quad (A1)$$

neglecting  $O(V_{ac}^2)$ .  $C_T = [\epsilon_0^{-1}(d + h_0) + \epsilon_{SiO_2}^{-1}t_{SiO_2}]^{-1}$  is the total effective capacitance (per unit area) due to the back-gate oxide and air dielectric.  $d$  is the perpendicular distance of graphene from the substrate when unstrained.

## APPENDIX B: ELASTIC FORCES

The position of a 2D membrane can be described by the in-plane and out-of-plane deformation field given by  $\mathbf{u}(x, y) = [u_x(x, y), u_y(x, y)]$  and  $h(x, y)$ . In the linear approximation, the strain tensor is given by,

$$u_{\alpha\beta} = \frac{1}{2}(\partial_\alpha u_\beta + \partial_\beta u_\alpha + \partial_\alpha \partial_\beta h) \quad (B1)$$

The elastic free energy is given by [6, 7],

$$\begin{aligned} \mathcal{E} &= \int dx dy \left[ \frac{1}{2} \kappa (\nabla^2 h)^2 + \frac{1}{2} \lambda (u_{xx} + u_{yy})^2 + \mu (u_{xx}^2 + u_{yy}^2 + 2u_{xy}^2) - \mathcal{F}_E^{eq} h \right] \\ &\approx \int dx \left[ \frac{1}{2} \kappa (\nabla^2 h)^2 + \frac{1}{2} (\lambda + 2\mu) u_{xx}^2 - \mathcal{F}_E^{eq} h \right] \end{aligned} \quad (B2)$$

where  $\kappa \approx 1\text{eV}$  is the bending rigidity,  $\mu \approx 9\text{eV}\text{\AA}^{-2}$  and  $\lambda \approx 2\text{eV}\text{\AA}^{-2}$  are the Lamé constants of graphene. Experiments [8] measures an elastic constant for graphite  $c_{11} = 106 \times 10^{10} \text{Nm}^{-2} \approx 1\text{TPa}$ . For graphene, we have the relation  $c_{11}d_{in} = \lambda + 2\mu$ . Using an interlayer separation distance of  $d_{in} = 0.335\text{nm}$  [9], we  $c_{11}d_{in} \approx 355\text{Nm}^{-1}$ . This is in good agreement with the values of Lamé constants we assumed. Recent measurement [10] of the Young's modulus of graphene yields  $E_{2d} = 342\text{Nm}^{-1}$ . Note that by definition,  $E_{2d} = c_{11}d_{in}$ .

$\mathcal{F}_E^{eq}$  is the pressure induced by the bottom electrostatic gate. Assuming homogeneity along transverse direction, we arrive to a one-dimensional problem. Minimizing  $\mathcal{E}$  in Eq. B2 yields us the following Euler-Lagrange equations,

$$\begin{aligned} \kappa \partial_x^4 h - (\lambda + 2\mu) \left[ \frac{3}{2} (\partial_x h)^2 \partial_x^2 h + \partial_x u_x \partial_x^2 h + \partial_x h \partial_x^2 u_x \right] &= \mathcal{F}_E^{eq} \\ \partial_x^2 u_x + \partial_x h \partial_x^2 h &= 0 \end{aligned} \quad (B3)$$

where the latter implies the longitudinal strain is constant i.e.

$$u_{xx} = \text{constant} \quad (\text{B4})$$

Finally, the differential equation governing  $h(x)$  is,

$$\kappa \partial_x^4 h - (\lambda + 2\mu) u_{xx} \partial_x^2 h = \mathcal{F}_E^{eq} \quad (\text{B5})$$

The differential equation for  $h$  then reduces to,

$$-(\lambda + 2\mu) u_{xx} \partial_x^2 h = \mathcal{F}_E^{eq} \quad (\text{B6})$$

whose explicit solution with the boundary condition  $h(\pm L/2) = 0$  is,

$$h(x) \approx \frac{\mathcal{F}_E^{eq}(L^2 - 4x^2)}{8(\lambda + 2\mu)u_{xx}} \equiv h_0 - \frac{4h_0}{L^2}x^2 \quad \text{where } h_0 = \frac{\mathcal{F}_E^{eq}L^2}{8(\lambda + 2\mu)u_{xx}} \quad (\text{B7})$$

where  $h_0$  is the maximum deflection i.e. at  $x = 0$ . Including the second order terms, the expression can be rather complicated [11]. With the profile  $h(x)$ , simple geometry allows us to relate  $u_{xx}$  with  $h_0$  as per Eq. C9. Then the elastic force equation reduces from Eq. B6 to,

$$\mathcal{F}_S^{eq} = -\frac{64}{3}(\lambda + 2\mu)\frac{h_0^3}{L^4} + \frac{8\Delta L}{L^3}(\lambda + 2\mu)h_0 = \mathcal{F}_E^{eq} \quad (\text{B8})$$

where we included the possibility of an initial tension,  $\Delta L < 0$ . Elastic forces due to deformation  $a$  away from the equilibrium can then be described by,

$$\mathcal{F}_S = -\frac{64}{3}\frac{\lambda + 2\mu}{L^4}(a^3 + 3a^2h_0 + 3ah_0^2) + \frac{8\Delta L}{L^3}(\lambda + 2\mu)a \quad (\text{B9})$$

### APPENDIX C: DEFORMATION AND GATING

Next we shall determine  $u_{xx}$ . Following [12], it is defined as,

$$u_{xx} = \frac{L' - (L + \Delta L)}{L + \Delta L} \approx \frac{L' - L}{L} - \frac{\Delta L}{L} \quad (\text{C1})$$

where  $L'$  is the length of the strained graphene,

$$L' = 2 \int_0^{L/2} dx \sqrt{1 + |\nabla h|^2} \approx L + \int_0^{L/2} dx (\partial_x h)^2 = \frac{L^3(\mathcal{F}_E^{eq})^2}{24(\lambda + 2\mu)^2 u_{xx}^2} + L \quad (\text{C2})$$

$L$  is trench length and  $L + \Delta L$  is length in absense of strain. Hence, solving  $u_{xx}$  then reduces to finding the root of,

$$u_{xx}^3 + \frac{\Delta L}{L}u_{xx}^2 - \frac{L^2(\mathcal{F}_E^{eq})^2}{24(\lambda + 2\mu)^2} = 0 \quad (\text{C3})$$

**No initial tension or slack:** If  $\Delta L = 0$ , we will obtain,

$$u_{xx} = \left[ \frac{L^2(\mathcal{F}_E^{eq})^2}{24(\lambda + 2\mu)^2} \right]^{1/3} = \frac{8h^2}{3L^2} \quad (\text{C4})$$

Electrostatically, one can approximate  $\mathcal{F}_E^{eq}$  as,

$$\mathcal{F}_E^{eq} \approx \frac{e^2 n^2}{2\epsilon_{eff}} \quad (\text{C5})$$

where  $n$  is the carrier density in graphene and  $\epsilon_{eff}$  is the effective dielectric due to air gap and back gate oxide. We ignore the curvature of graphene. Assuming that  $\Delta L = 0$ , we get an expression for maximum deflection  $h_0$  at equilibrium,

$$h_0 = \left[ \frac{3L^4 e^2 n^2}{128 \epsilon_{eff} (\lambda + \mu)} \right]^{\frac{1}{3}} \quad (C6)$$

**With initial tension or slack:** For general case of  $\Delta L \neq 0$ , To obtain  $h_0$  rigorously requires solving the following the electrostatic and elasticity equations self-consistently.

$$F_E^{eq} = \frac{1}{2\epsilon_0} \left[ \left( \frac{\overbrace{\epsilon_0}^{C_a}}{d - h_0} \right)^{-1} + \left( \frac{\overbrace{\epsilon_{ox}}^{C_{ox}}}{t_{ox}} \right)^{-1} \right]^{-2} V_{dc}^2 \quad (C7)$$

$$-\frac{64}{3L^3} h_0^3 + \frac{8\Delta L}{L^2} h_0 + \frac{F_E^{eq} L}{\lambda + 2\mu} = 0 \quad (C8)$$

When  $F_E^{eq} = 0$ , the latter requires  $h_0 = 0$  for  $\Delta L \leq 0$  (tension), which is expected. Another remark. A series capacitance  $C_{ox}$  to  $C_a$  is essential as it provides stability to the electrically actuated mechanical system. A relation between  $u_{xx}$  and  $h_0$  can be obtained from Eq. B7 and C3, yielding,

$$\begin{aligned} u_{xx}^3 + \left( \frac{\Delta L}{L} - \frac{8h_0^2}{3L^2} \right) u_{xx}^2 &= 0 \\ \Rightarrow u_{xx} = 0 \text{ or } u_{xx} &= \frac{8h_0^2}{3L^2} - \frac{\Delta L}{L} \end{aligned} \quad (C9)$$

- 
- [1] J. S. Bunch, A. M. Zande, S. S. Verbridge, I. W. Frank, D. M. Tanenbaum, J. M. Parpia, H. G. Craighead, and P. L. McEuen, "Electromechanical resonator from graphene sheets," *Science*, vol. 315, p. 490, 2007.
  - [2] C. Chen, S. Rosenblatt, K. I. Bolotin, W. Kalb, P. Kim, I. Kymissis, H. L. Stormer, T. F. Heinz, and J. Hone, "Performance of monolayer graphene nanomechanical resonators with electrical readout," *Nature Nano.*, vol. 4, p. 861, 2009.
  - [3] A. Eichler, J. Moser, J. Chaste, M. Zdrojek, I. W. Rae, and A. Bachtold, "Nonlinear damping in mechanical resonators based on graphene and carbon nanotubes," *arXiv:1103.1788*, 2011.
  - [4] W. T. Thomson and M. D. Dahleh, "Theory of vibrations with applications," *Prentice Hall*, 1997.
  - [5] G. Duffing, "Erzwungene schwingungen bei vera?nderlicher eigenfrequenz und ihre technische bedeutung," *Braunschweig Vieweg*, 1918.
  - [6] M. A. H. Vozmediano, M. I. Katsnelson, and F. Guinea, "Gauge fields in graphene," *Phys. Rep.*, vol. 496, p. 109, 2010.
  - [7] L. D. Landau and E. M. Lifshitz, "Theory of elasticity," *Pergamon Press*, 1986.
  - [8] O. L. Blakslee, D. G. Proctor, E. J. Seldin, G. B. Spence, and T. Weng, "Elastic constants of compression annealed pyrolytic graphite," *J. Appl. Phys.*, vol. 41, p. 3373, 1970.
  - [9] R. Al-Jishi and G. Dresselhaus, "Lattice dynamical model for graphite," *Phys. Rev. B*, vol. 26, p. 4514, 1982.
  - [10] C. Lee, X. Wei, J. W. Kysar, and J. Hone, "Measurement of the elasti properties and intrinsic strength of monolayer graphene," *Science*, vol. 321, p. 385, 2008.
  - [11] S. P. Timoshenko and S. Woinowsky-Kreiger, "Theory of plates and shells," *McGraw Hill, New York*, 1959.
  - [12] M. M. Fogler, F. Guinea, and M. I. Katsnelson, "Pseudomagnetic fields and ballistic transport in a suspended graphene sheet," *Phys. Rev. Lett.*, vol. 101, p. 226804, 2008.
